# Supplementary material for: Spin-wave emission with current-controlled frequency by a PMA-based spin-Hall oscillator
Source: arXiv:2512.00593 ancillary file (2026-03-06)
Supplement: Supplementary file 1 [file 20251129_Supplement.pdf]

## Supplemental Material

-

### Spin-wave emission with current-controlled frequency by a PMA-based spin-Hall oscillator

M. Bechberger,<sup>1, a)</sup> D. Breitbach,<sup>1, a)</sup> A. Koujok,<sup>1</sup> B. Heinz,<sup>1</sup> C. Dubs,<sup>2</sup> A. Hamadeh,<sup>3</sup>  
and P. Pirro<sup>1</sup>

<sup>1)</sup>*Fachbereich Physik and Landesforschungszentrum OPTIMAS,  
Rheinland-Pfälzische Technische Universität Kaiserslautern-Landau,  
D-67663 Kaiserslautern, Germany*

<sup>2)</sup>*INNOVENT e.V. Technologieentwicklung, D-07745 Jena, Germany*

<sup>3)</sup>*Université Paris-Saclay, Centre de Nanosciences et de Nanotechnologies,  
CNRS, 91120, Palaiseau, France*

(\*Electronic mail: [mbechber@rptu.de](mailto:mbechber@rptu.de))

(Dated: 29 November 2025)

---

<sup>a)</sup>M. Bechberger and D. Breitbach contributed equally to this work.

## Contents

|                                                              |   |
|--------------------------------------------------------------|---|
| <b>I. Calculation of the nonlinear frequency shift</b>       | 2 |
| <b>II. FMR measurements on full-film reference samples</b>   | 3 |
| A. Ga:YIG                                                    | 4 |
| B. Influence of Pt layer                                     | 5 |
| <b>III. Calculated dispersion relation and mode profiles</b> | 7 |
| <b>IV. Reciprocal spin-wave emission</b>                     | 8 |
| <b>V. Micromagnetic simulations</b>                          | 8 |
| A. Simulation setup                                          | 8 |
| B. Application of negative current values                    | 9 |

### I. Calculation of the nonlinear frequency shift

The Hamiltonian framework for nonlinear spin-wave theory<sup>1</sup> gives access to the calculation of the nonlinear frequency shift in Ga:YIG by providing the linear eigenfrequency and the coefficients for self- and cross-nonlinear frequency shifts required to determine the modified frequency at finite spin-wave intensities. The magnetic film is characterized by its thickness  $t$ , saturation magnetization  $M_s$ , and exchange constant  $A = 1.35 \text{ pJ m}^{-1}$ . These values define an exchange length  $\lambda_{\text{ex}} = \sqrt{2A/(\mu_0 M_s^2)}$ . The out-of-plane uniaxial anisotropy constant  $K_u$  defines the anisotropy field  $\mu_0 H_u = 2K_u/M_s$ . Since Ga:YIG exhibits a dominant  $H_u$  and appears to be almost isotropic, the cubic anisotropy is not considered in the following. An external field  $H_{\text{ext}}$  is applied under the angle  $\theta_H$  to the film normal, leading to a specific magnetization angle  $\theta_M$ , which can be determined via the following equation<sup>1</sup>:

$$H_{\text{ext}} \sin(\theta_M - \theta_H) = \frac{M_{\text{eff}}}{2} \sin(2\theta_M), \quad (\text{S1})$$

with  $M_{\text{eff}} = M_s - H_u$ . Analogous to our experimental setup, we set  $\mathbf{H}_{\text{ext}} = H_{\text{ext}} \hat{\mathbf{e}}_x$  with  $\theta_H = 90^\circ$  and the equation is solved numerically. The equilibrium orientation  $\theta_M$  gives rise to the internal

effective magnetic field  $\mathbf{H}_{\text{int}}$ , which can be derived from:

$$\mathbf{H}_{\text{int}} = \frac{1}{\mu_0} \frac{\delta \varepsilon}{\delta \mathbf{M}} = H_{\text{ext}} \hat{\mathbf{e}}_x + \left( \frac{H_u}{M_s} - N_{zz} \right) M_s \cos(\theta_M) \hat{\mathbf{e}}_z. \quad (\text{S2})$$

In the case of a thin film the out-of-plane demagnetization factor can be approximated by  $N_{zz} \approx 1$ , allowing for following intermediate expressions

$$Q_k = \frac{\omega_M}{2} \left( 2\lambda_{\text{ex}}^2 k^2 + \left( 1 - \frac{H_U}{M_S} \right) \sin^2 \theta_M \right),$$

$$B_k = \frac{\omega_M}{2} \left( \left( \frac{H_U}{M_S} - 1 \right) \sin^2 \theta_M \right), \quad (\text{S3})$$

$$\Gamma_{zz,k} = \omega_M \left( \lambda_{\text{ex}}^2 k^2 + \left( 1 - \frac{H_U}{M_S} \right) \cos^2 \theta_M \right), \quad (\text{S4})$$

with  $\omega_M = \gamma \mu_0 M_s$  and  $\omega_H = \gamma \mu_0 H_{\text{int}}$ . The spin-wave eigenfrequency of mode  $k$  is given by  $\omega_k = \sqrt{(\omega_H + Q_k)^2 - |B_k|^2}$ . In this study, it is appropriate to simplify to the case of  $k \rightarrow 0$ , since this mode corresponds to the minimum frequency and is dominantly populated by the injected spin current, causing an auto-oscillation. Its nonlinearly shifted spin-wave frequency  $\tilde{\omega}_0$  is in the underlying case influenced by the nonlinear self-shift caused through its own spin-wave intensity  $|c_0|^2$ , which is defined by the self-shift coefficient

$$N = -Q_0 + \frac{B_0^2}{2\omega_0^2} \omega_H + \left( 1 + \frac{3B_0^2}{2\omega_0^2} \right) \Gamma_{zz,0}. \quad (\text{S5})$$

## II. FMR measurements on full-film reference samples

This section characterizes the magnetic properties of Ga:YIG<sup>2</sup> and quantifies the influence of the additional platinum layer by using ferromagnetic resonance (FMR) spectroscopy, which is based on the resonant absorption of an alternating microwave field by the magnetic sample. In this study, the excitation frequency is swept for a constant magnetic field, and excitation as well as detection is accomplished by a vector network analyzer (VNA). The analysis is simplified, as the cubic anisotropy is assumed to be negligible, an assumption that seems reasonable given the known values for comparable Ga:YIG samples with  $|H_C| < 5 \text{ mT}$ <sup>3,4</sup>. Therefore, the mathematical description of the FMR frequency  $f_{\text{FMR}}$  of the in-plane magnetized Ga:YIG film on a GGG substrate in (111) orientation is independent of the crystallographic axis' orientation and given by

$$f_{\text{FMR}} = |\gamma| \mu_0 \sqrt{H_{\text{ext}} \cdot (H_{\text{ext}} + M_{\text{eff}})}, \quad (\text{S6})$$

with an effective magnetization of

$$M_{\text{eff}} = M_S - H_U. \quad (\text{S7})$$

Equation S6 can be applied to the extracted resonance frequencies as a function of the external field, which gives access to  $M_{\text{eff}}$ . Under the assumption that the saturation magnetization  $M_S$ , which was obtained by vibrating sample magnetometry (VSM), is known, Eq. S7 allows for the extraction of the uniaxial anisotropy  $H_U$ . Furthermore, the extraction of the resonance frequency provides additional insight via its frequency linewidth, as it can be converted to a field linewidth

$$\Delta H = \Delta \omega_{\text{FMR}} \left( \frac{\partial H_{\text{ext}}(\omega_{\text{FMR}})}{\partial \omega_{\text{FMR}}} \right) = \Delta \omega_{\text{FMR}} \left( \frac{\partial \omega_{\text{FMR}}}{\partial H_{\text{ext}}(\omega_{\text{FMR}})} \right)^{-1}, \quad (\text{S8})$$

which is directly related to the Gilbert damping parameter  $\alpha$ :

$$\alpha = \frac{|\gamma| \mu_0 \Delta H}{2 f_0}. \quad (\text{S9})$$

Therefore, the Gilbert damping parameter can also be extracted from this measurement by applying a linear fit to  $\mu_0 \Delta H$  as a function of  $f_{\text{FMR}}$ . It should be noted that the non-viscous contributions are not considered for  $\alpha$ , which can be estimated via the inhomogeneous field linewidth  $\mu_0 \Delta H(f_{\text{FMR}} = 0)$ , serving as measure for the inhomogeneity of the sample.

Given that the investigated and fabricated sample only consists of a vanishing magnetic volume, it is necessary to use full-film reference samples instead. Therefore, the characterization of Ga:YIG is performed using a sample that originates from the same material wafer as the sample under study. However, for the quantification of the influence induced by a thin platinum layer two Ga:YIG films from another material wafer with comparable material parameters are used.

## A. Ga:YIG

The FMR measurement of the bare Ga:YIG film, which serves as a direct reference to the sample under study, was performed by applying the external field along both relevant crystallographic axes,  $[1\bar{1}0]$  and  $[11\bar{2}]$ . Figure S1 (a) depicts the extracted resonance frequency  $f_{\text{FMR}}$  as a function of the external magnetic field  $\mu_0 H_{\text{ext}}$ , with the field oriented along the  $[1\bar{1}0]$  crystallographic axis, a configuration that has been demonstrated to be more accurate in extracting  $M_{\text{eff}}$ <sup>4</sup>. The application of Eq. S6 yields  $\gamma = 28.63 \text{ GHz T}^{-1}$  and  $M_{\text{eff}} = -74.4 \text{ mT}$ . Given the value  $M_S = 20.38 \text{ mT}$ , obtained via VSM, an uniaxial anisotropy of  $H_U = 94.78 \text{ mT}$  can be extracted using Eq. S7, which aligns with Ga:YIG material parameters of the most recent studies. Figure S1 (b)

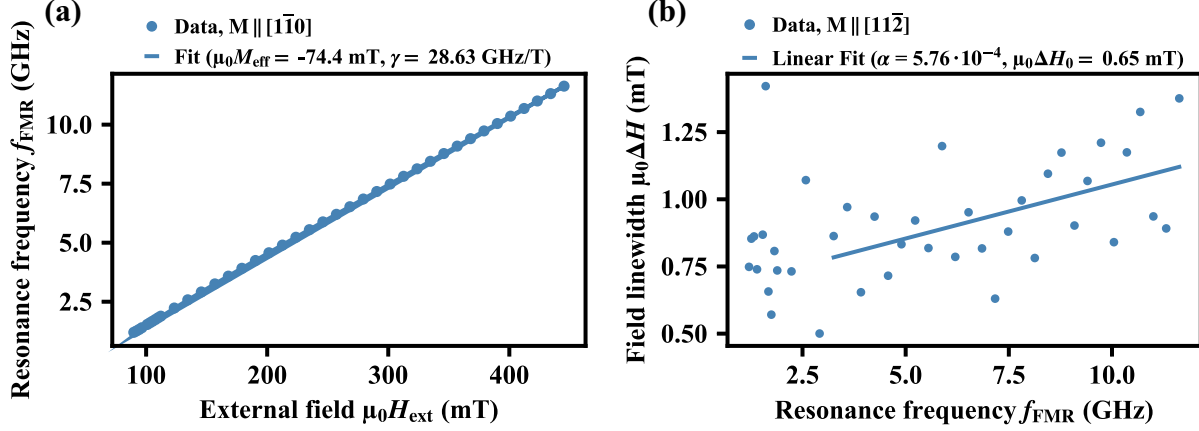

FIG. S1. FMR spectroscopy on Ga:YIG (a) Extracted resonance frequency as a function of the external magnetic field for the Ga:YIG full film reference sample along the  $[1\bar{1}0]$  crystallographic axis. The Kittel fit function according to Eq. S6 is applied to the data. (b) Extracted field linewidth as a function of the resonance frequency for the similar film but along the  $[11\bar{2}]$  crystallographic axis. A linear fit is applied, from which  $\alpha$  can be extracted through Eq. S8.

depicts the field linewidth  $\mu_0 \Delta H$  as a function of the resonance frequency  $f_{\text{FMR}}$ , with the field oriented along the  $[11\bar{2}]$  crystallographic axis, as this configuration is used for the study of the fabricated sample. While the linewidth data is noisy, the application of Eq. S8 allows for a rough determination of the Gilbert damping parameter, or at least its order of magnitude, yielding a value of  $\alpha = 5.76 \times 10^{-4}$  and an inhomogeneous field linewidth of  $\mu_0 \Delta H_0 = 0.65$  mT. While  $\alpha$  aligns with the value determined on a comparable Ga:YIG thin film from the aforementioned studies,  $\mu_0 \Delta H_0$  is increased. Therefore, it can be concluded that the recently fabricated Ga:YIG thin films exhibit greater inhomogeneity compared to the well-established YIG thin films<sup>5</sup>.

## B. Influence of Pt layer

The following FMR measurements were performed on a Ga:YIG and Ga:YIG/Pt thin film, which originate from the same material wafer and exhibit comparable characteristics as the sample under study. The thickness of 56 nm and the determined value  $M_S = 20.23$  mT of the bare Ga:YIG film, which has been obtained via VSM, emphasize their comparability. The platinum layer of the reference sample was deposited during the same process as the fabricated sample under study to allow for direct comparison between the samples regarding the influence of the platinum layer. Figure S2 (a) depicts the extracted resonance frequency  $f_{\text{FMR}}$  as a function of

the external magnetic field  $\mu_0 H_{\text{ext}}$ , with the field oriented along both crystallographic axes for Ga:YIG and along  $[1\bar{1}0]$  for Ga:YIG/Pt. The comparison of Ga:YIG along the two axes reveals a discrepancy that emerges for fields approaching the absolute value of  $\mu_0 M_{\text{eff}}$ . Along  $[11\bar{2}]$ , a saturation at a finite frequency occurs, which has been attributed to a slower dragging of the magnetization into the plane compared to the other axis orientation<sup>4</sup>. Therefore, the configuration along  $[11\bar{2}]$  is not the optimal choice for extracting  $M_{\text{eff}}$ , yet it is included here to demonstrate the feasibility of approximating it via a quadratic fit function around the minimum frequency. While the more reliable application of Eq. S6 to the data along  $[1\bar{1}0]$  yields  $\gamma = 28.68 \text{ GHz T}^{-1}$  and  $M_{\text{eff,Ga:YIG}} = -72.5 \text{ mT}$ , the minimum frequency for the measurement along  $[11\bar{2}]$  is situated at the compensation field  $H_{\text{comp}} = 75.26 \text{ mT}$ . Consequently, an error of around 3 mT is present for the approximation via  $H_{\text{comp}}$ . The extraction of  $M_{\text{eff,Ga:YIG/Pt}} = -69.66 \text{ mT}$  for the Ga:YIG/Pt

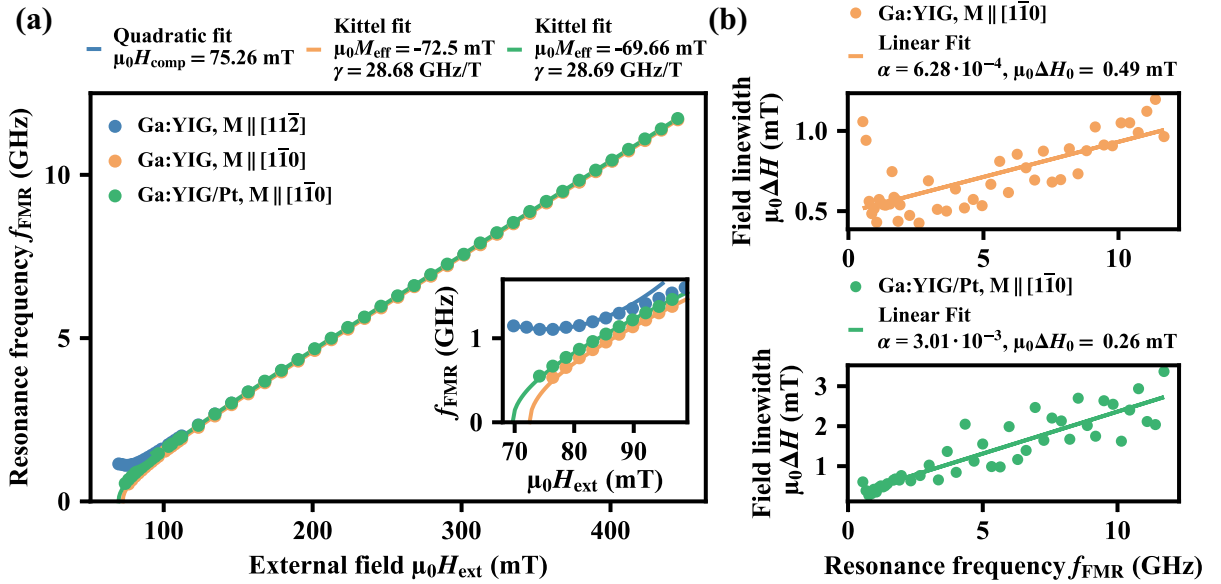

FIG. S2. FMR spectroscopy on Ga:YIG/Pt (a) Extracted resonance frequency as a function of the external magnetic field for a Ga:YIG thin film long both crystallographic axes and for a Ga:YIG/Pt thin film along  $[1\bar{1}0]$ . The inset is included for better visualization of the low-field regime. A quadratic fit is applied to the data  $\mathbf{M} \parallel [11\bar{2}]$  up to fields of 90 mT and the Kittel formula according to Eq. S6 is applied on the data for  $\mathbf{M} \parallel [11\bar{2}]$ . (b) The two graphs depict the extracted field linewidth as a function of the resonance frequency for Ga:YIG and Ga:YIG/Pt. Linear fits are applied, from which  $\alpha$  can be extracted through Eq. S8.

film yields an absolute reduction of around 3 mT compared to its Ga:YIG reference, which can be attributed to the change in anisotropy under the assumption that  $M_S$  remains constant. Conse-

quently, according to the full-film reference study, the material systems Ga:YIG/Pt and Ga:YIG demonstrate comparable frequencies during investigations at a constant field, suggesting that they can be treated approximately identically. However, the evaluation of the Gilbert damping parameter of both material systems reveals a five-fold enhancement from  $\alpha_{\text{Ga:YIG}} = 6.28 \times 10^{-4}$  to  $\alpha_{\text{Ga:YIG/Pt}} = 3.01 \times 10^{-3}$ , which can be attributed to the presence of the platinum layer. This phenomenon had previously been observed in YIG/Pt, where enhancement by an order of magnitude was observed, with the spin-pump effect identified as the main mechanism<sup>6</sup>.

### III. Calculated dispersion relation and mode profiles

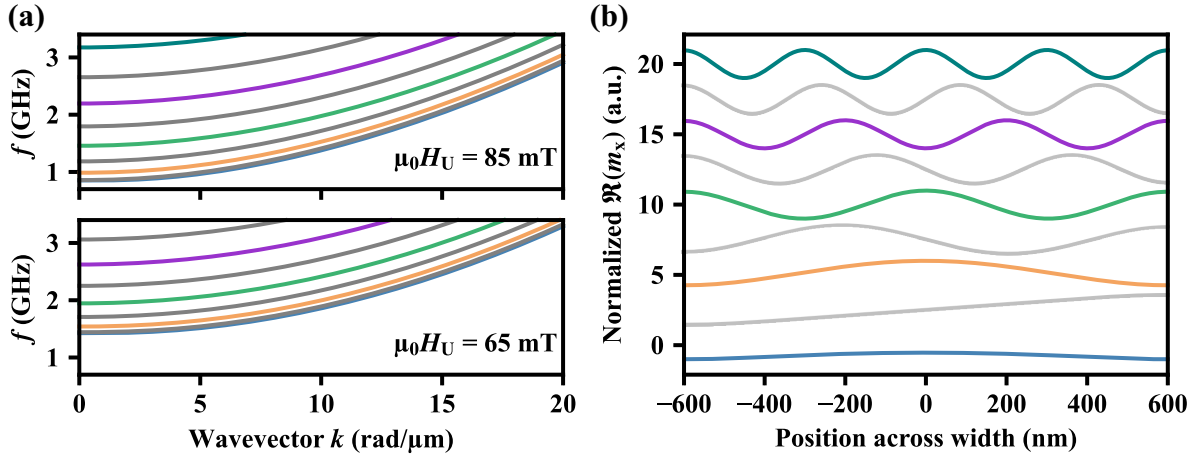

FIG. S3. Dispersion relation and mode profiles of Ga:YIG **(a)** Calculated spin-wave dispersion for the fundamental and strain mode for an external field of  $\mu_0 H_{\text{ext}} = 77.46$  mT. **(b)** Extracted mode profiles are shown in (a) with artificial offset for each mode to improve visibility.

The spin-wave dispersion relation in the Ga:YIG waveguide with the respective waveguide mode profiles are calculated using the open-source TetraX finite-element micromagnetic modeling package<sup>7,8</sup>. The material parameters used are the thickness  $t = 55$  nm, the width  $w = 1.2 \mu\text{m}$ ,  $\mu_0 M_S = 20.38$  mT,  $A = 1.35$  pJ m<sup>-1</sup> and the two determined uniaxial anisotropies  $H_{U,\text{Ga:YIG}} = 85$  mT and  $H_{U,\text{edge}} = 65$  mT. The dispersion relations of the center and edge region are shown in Fig. S3 (a) for  $\mu_0 H_{\text{ext}} = 77.46$  mT, including the higher modes up to a frequency of 3.5 GHz. The gray lines correspond to the odd modes, which exhibit a vanishing total magnetization across the waveguide width, as shown by the mode profiles in Fig. S3 (b). The two fundamental modes at  $k = 0$  of both regions align with the frequency of the two distinct modes measured on Ga:YIG/Pt

(see main manuscript). Despite the higher modes remaining undetected in thermal measurements, multiple modes are excited via SOT. These correspond approximately to higher modes for  $k = 0$  shown in Fig. S3 (a). Note that the excited frequencies of the higher modes may correspond to modes from both the fundamental and edge mode.

#### IV. Reciprocal spin-wave emission

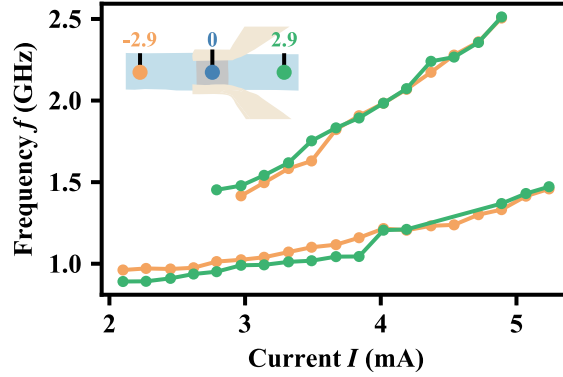

FIG. S4. Reciprocal emission. Extracted frequencies from BLS measurements obtained in a distance of 2.9  $\mu\text{m}$  to the Pt pad, as indicated in the pictogram.

In order to investigate the reciprocal emission of spin waves, two BLS measurements are performed at a distance of 2.9  $\mu\text{m}$  in both directions from the Pt pad, as indicated by the colored dots in the schematic of Fig. S4. The extracted frequencies of the two propagating modes are shown as a function of the applied DC current  $I$ , demonstrating the reciprocal character of the emission.

#### V. Micromagnetic simulations

The micromagnetic study is performed using the open-source micromagnetic solver MuMax 3.0 package<sup>9</sup>, as well as the compute platform Aithericon<sup>10</sup>.

##### A. Simulation setup

For the simulations, cell sizes of 10x10x55 nm<sup>3</sup> are selected, corresponding to 10 nm cells in the xy-plane and a single 55 nm cell in z. The sample dimensions are given by a total length in x of 10.24  $\mu\text{m}$ , a width in y of 1.2  $\mu\text{m}$  and a thickness in z of 55 nm. The damping towards both

ends along x is artificially increased by a hyperbolic function to minimize reflection and other influences by the finite system. The injection area for the spin current, which represents the Pt pad, is positioned in the center of the layout with a length along the x-direction of 1  $\mu\text{m}$ .

The Slonczewski model is used for the spin current with following parameters: Polarization  $P = 0.5669$ , secondary STT term  $\varepsilon' = 0$  and the Slonczewski parameter  $\Lambda = 1$ .

Following material parameters are used for the bare Ga:YIG region outside of this area, which were determined in the framework of this study:  $M_S = 16.202 \text{ kA m}^{-1}$ , exchange constant  $A_{\text{ex,Ga:YIG}} = \frac{1}{2} \lambda_{\text{ex,Ga:YIG}}^2 \mu_0 M_S^2 = 1.35 \text{ pJ m}^{-1}$ ,  $\alpha_{\text{Ga:YIG}} = 5.76 \times 10^{-4}$ , uniaxial anisotropy constant  $K_{\text{U,Ga:YIG}} = \mu_0 H_{\text{U,Ga:YIG}} \times \frac{M_S}{2}$  along z-direction. The external field is set to  $\mu_0 H_{\text{ext}} = 77.46 \text{ mT}$  and oriented along x-direction. The injection area exhibits an overall damping of  $5 \times \alpha_{\text{Ga:YIG}}$ , which is in accordance with the findings from Sec. II. To account for the magnetically inhomogeneous Pt pad, three regions varying in  $K_U$  are defined. The center region is represented by the fundamental mode excitation, which aligns approximately with the bare Ga:YIG in the experiment, and is therefore set to  $\mu_0 H_{\text{U,Ga:YIG}} = 85 \text{ mT}$ . Only the two edge regions are defined with the changed anisotropy of  $\mu_0 H_{\text{U,edge}} = 65 \text{ mT}$ . The setup corresponds to the most simplistic model for an inhomogeneous anisotropy, with a symmetric geometry, in order to reproduce the experiment and underline the assumptions made in the main manuscript.

The data presented in the manuscript, derived from micromagnetic simulations, are obtained by performing a fast Fourier transform (FFT) of the magnetization component  $m_y$  as a function of time, averaged within a region of  $0.2 \times 0.2 \mu\text{m}^2$ .

## B. Application of negative current values

The simulated Fourier spectra  $\mathcal{F}(m_y(t))$  in the main manuscript are shown as a function of the current density  $j$  within the positive regime, corresponding to the anti-damping torque configuration. However, the damping torque and its influence on the spectrum can be studied by applying negative values  $j < 0$ , which is shown in Fig. S5. Figure S5 (a) depicts the entire range of current density values, demonstrating the asymmetry in excitation due to the spin Hall effect. In order to study the regime of the damping torque, this range is separately shown in Fig. S5 (b), making the spectrum visible. It is evident that the frequency remains constant at approximately 1 GHz, which corresponds to the frequency of the thermal spectrum. The experimentally observed frequency shift within the regime of the damping torque is not reproduced by simulations, which indicates

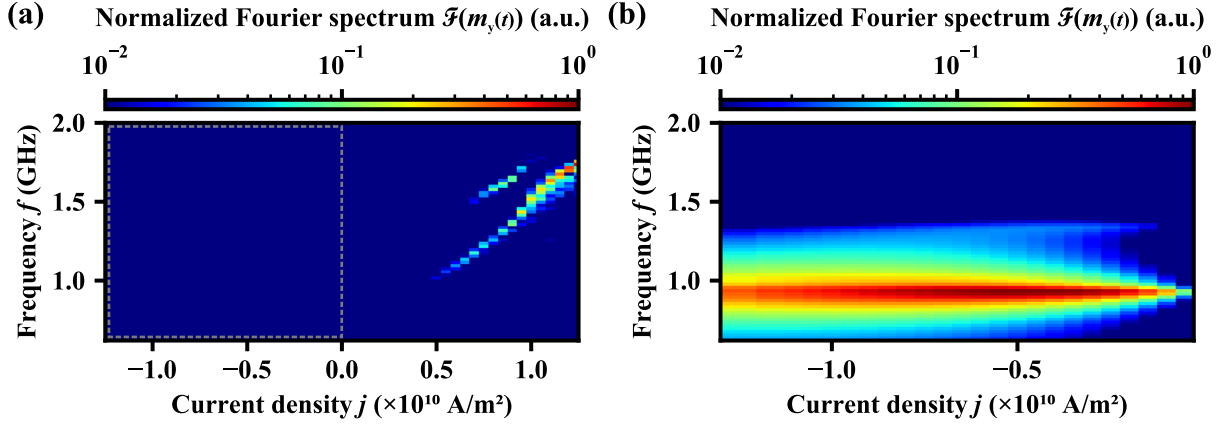

FIG. S5. Simulation in the damping-torque regime **(a)** and **(b)** Normalized Fourier spectrum  $\mathcal{F}(m_y(t))$  as a function of the current density  $j$ , obtained within the injection area for the magnetically inhomogeneous pad ( $w_{\text{edge}} = \frac{2}{5}b$ ). The gray dashed box represents the region of interest shown in **(b)**.

that heating influences the magnetic system. However, since the simulation of the SHO is mostly in agreement with the experimental observation, it can be concluded that heat or heat-induced strain is not the dominant effect for its operation.

## References

- <sup>1</sup>P. Krivosik and C. E. Patton, “Hamiltonian formulation of nonlinear spin-wave dynamics: Theory and applications,” [Physical Review B](#) **82**, 184428 (2010).
- <sup>2</sup>C. Dubs and O. Surzhenko, “Magnetically compensated nanometer-thin Ga-substituted yttrium iron garnet (Ga:YIG) films with robust perpendicular magnetic anisotropy,” [Advanced Electronic Materials](#) **11**, e00232 (2025).
- <sup>3</sup>T. Böttcher, M. Ruhwedel, K. O. Levchenko, Q. Wang, H. L. Chumak, M. A. Popov, I. V. Zavislyak, C. Dubs, O. Surzhenko, B. Hillebrands, A. V. Chumak, and P. Pirro, “Fast long-wavelength exchange spin waves in partially compensated Ga:YIG,” [Applied Physics Letters](#) **120**, 102401 (2022).
- <sup>4</sup>J. J. Carmiggelt, O. C. Dreijer, C. Dubs, O. Surzhenko, and T. van der Sar, “Electrical spectroscopy of the spin-wave dispersion and bistability in gallium-doped yttrium iron garnet,” [Applied Physics Letters](#) **119**, 202403 (2021).
- <sup>5</sup>C. Dubs, O. Surzhenko, R. Thomas, J. Osten, T. Schneider, K. Lenz, J. Grenzer, R. Hübner, and E. Wendler, “Low damping and microstructural perfection of sub-40nm-thin yttrium iron garnet

- films grown by liquid phase epitaxy,” [Phys. Rev. Mater. \*\*4\*\*, 024416 \(2020\)](#).
- <sup>6</sup>Y. Sun, H. Chang, M. Kabatek, Y.-Y. Song, Z. Wang, M. Jantz, W. Schneider, M. Wu, E. Montoya, B. Kardasz, B. Heinrich, S. G. E. te Velthuis, H. Schultheiss, and A. Hoffmann, “Damping in Yttrium Iron Garnet Nanoscale Films Capped by Platinum,” [Physical Review Letters \*\*111\*\*, 106601 \(2013\)](#).
- <sup>7</sup>L. Körber, G. Quasebarth, A. Otto, and A. Kákay, “Finite-element dynamic-matrix approach for spin-wave dispersions in magnonic waveguides with arbitrary cross section,” [AIP Advances \*\*11\*\*, 095006 \(2021\)](#).
- <sup>8</sup>L. Körber, G. Quasebarth, A. Hempel, F. Zahn, A. Otto, E. Westphal, R. Hertel, and A. Kakay, “[TetraX: Finite-Element Micromagnetic-Modeling Package](#),” (2022).
- <sup>9</sup>A. Vansteenkiste, J. Leliaert, M. Dvornik, M. Helsen, F. Garcia-Sanchez, and B. Van Waeyenberge, “The design and verification of MuMax3,” [AIP Advances \*\*4\*\*, 107133 \(2014\)](#).
- <sup>10</sup>for further details, “[www.aithericon.com](http://www.aithericon.com),”.
